# Supplementary material for: AutoEnRichness: A hybrid empirical and analytical approach for estimating the richness of galaxy clusters
Source: arXiv:2208.11944 source file (2022-08-25)
Supplement: Supplementary file 1 [file supplementary_material.pdf]

**Supplementary material (online)**

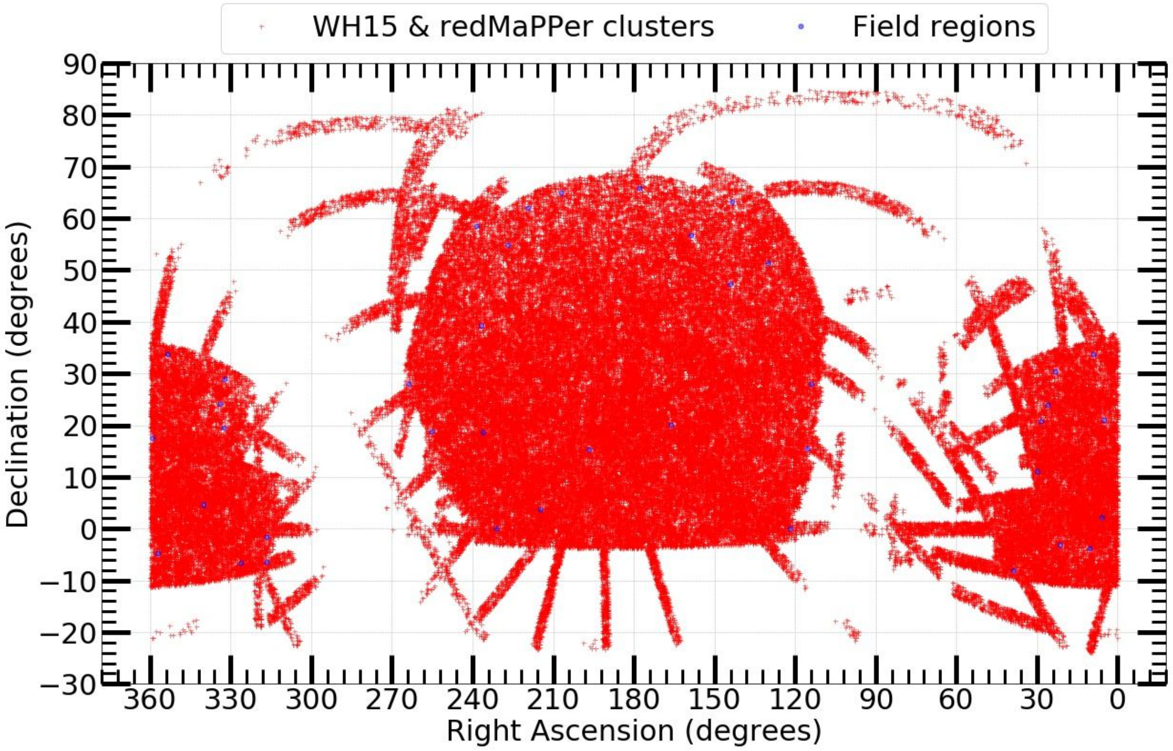


**Figure S1.** This figure displays a sky map of the astronomical coordinates (J2000) for the WH15 and redMaPPer clusters (red cross) as well as the astronomical coordinates of our forty different proposed ‘field’ regions (blue circle).

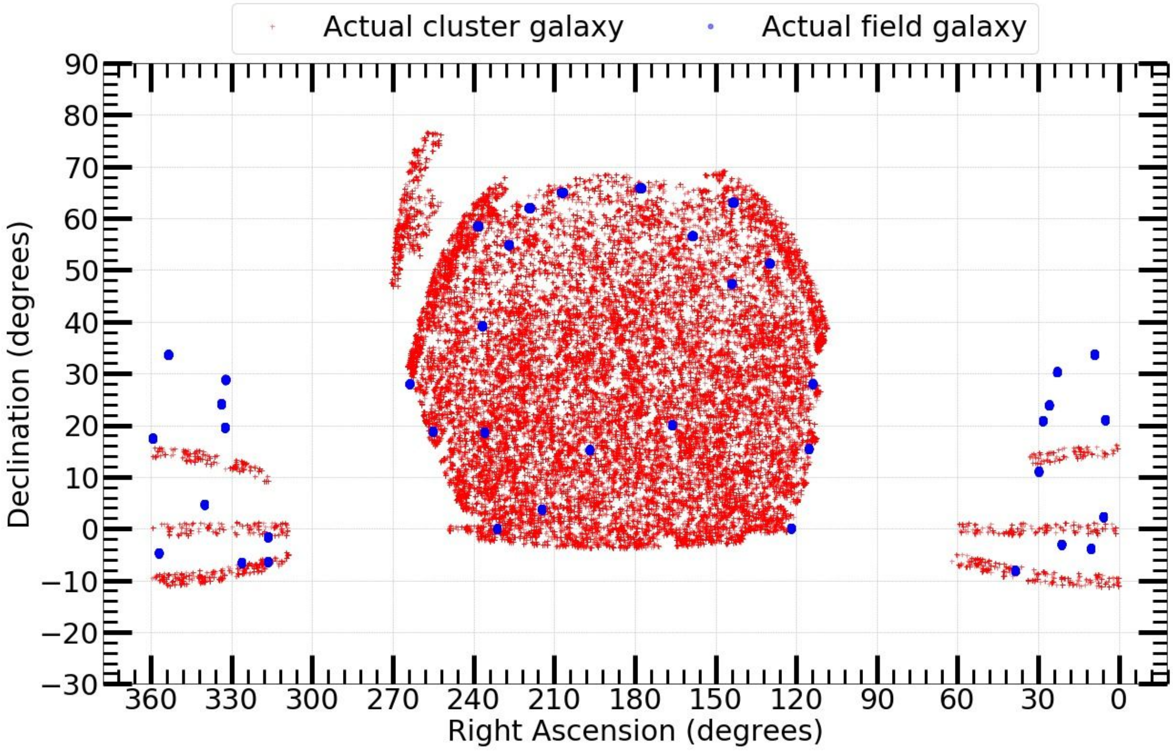


**Figure S2.** This figure displays a sky map of the astronomical coordinates (J2000) for the cluster (red cross) and field (blue circle) galaxies that had been cross-matched with galaxies observed within SDSS-IV DR16.

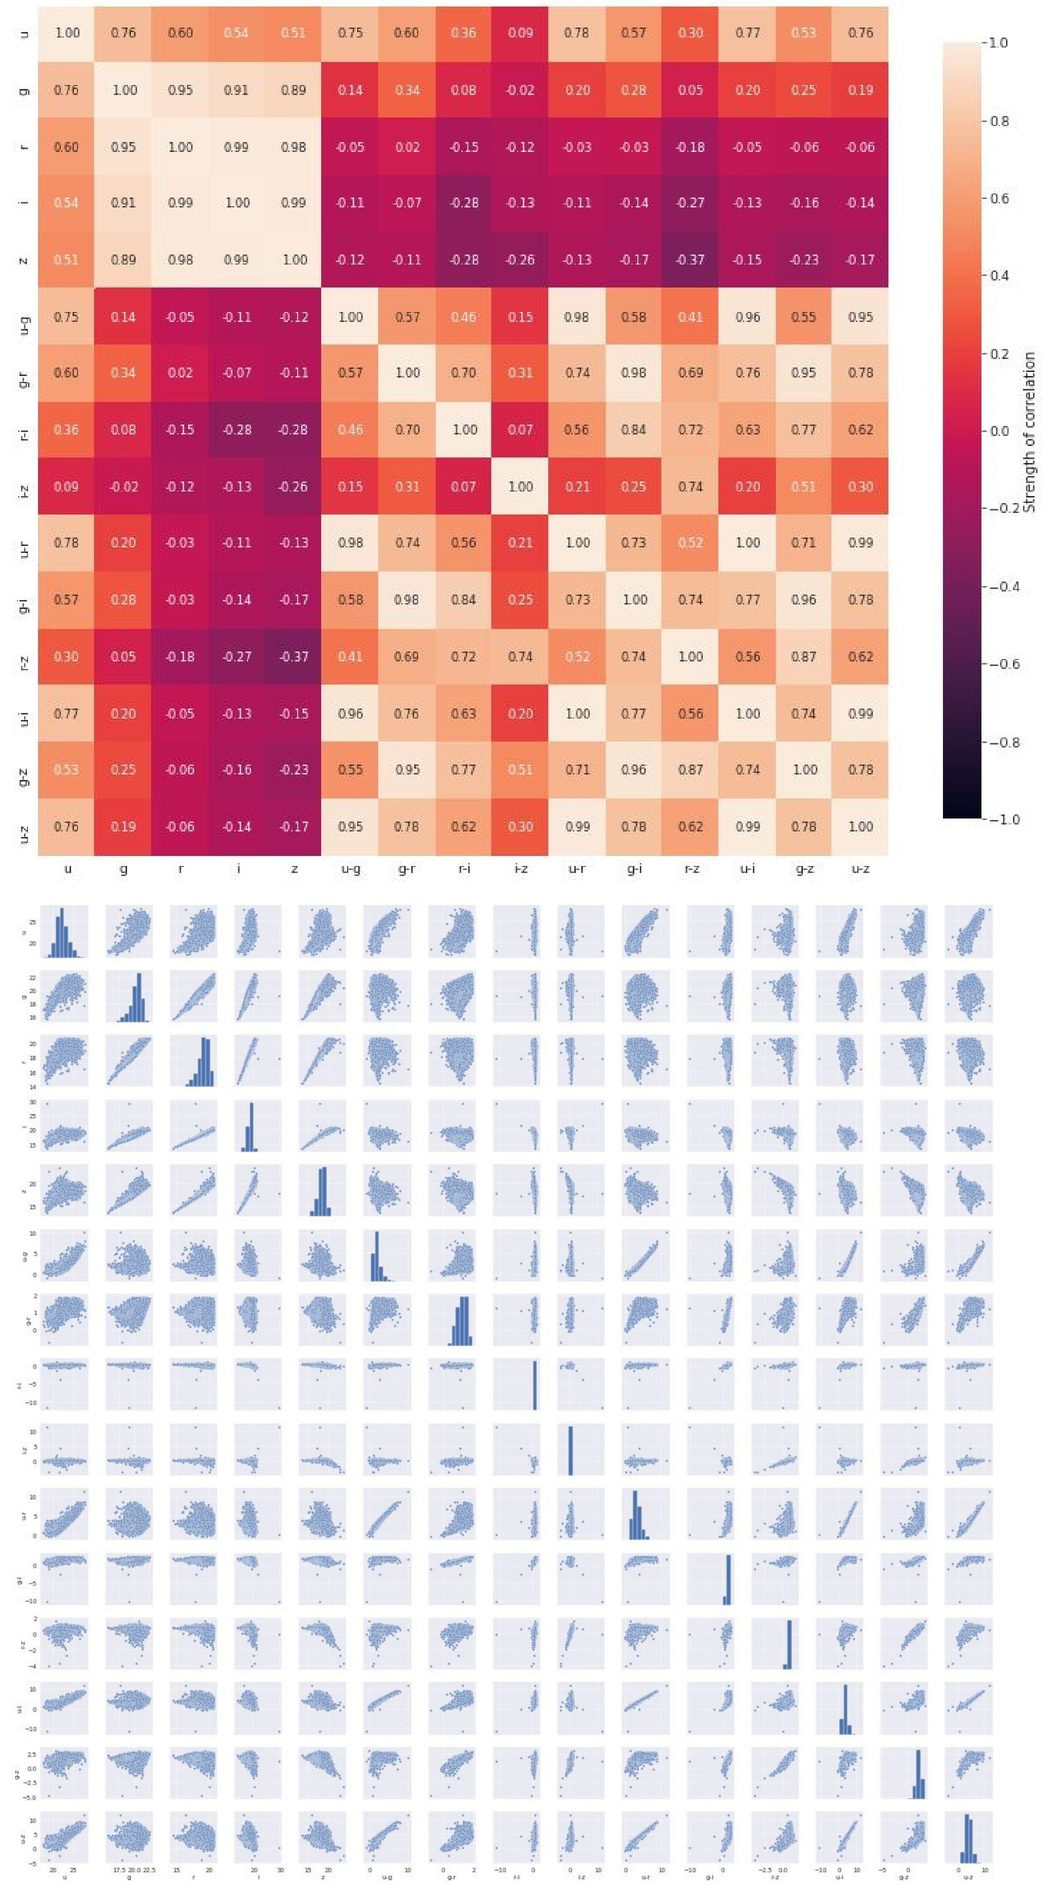


**Figure S3.** This figure displays a correlation matrix heatmap (top image) and scatterplots (bottom image) of features (i.e. filters and colours) from optical photometry data of galaxies in our cluster galaxy sample. The colourbar for the correlation matrix heatmap represents the strength and direction of the linear correlation between features.

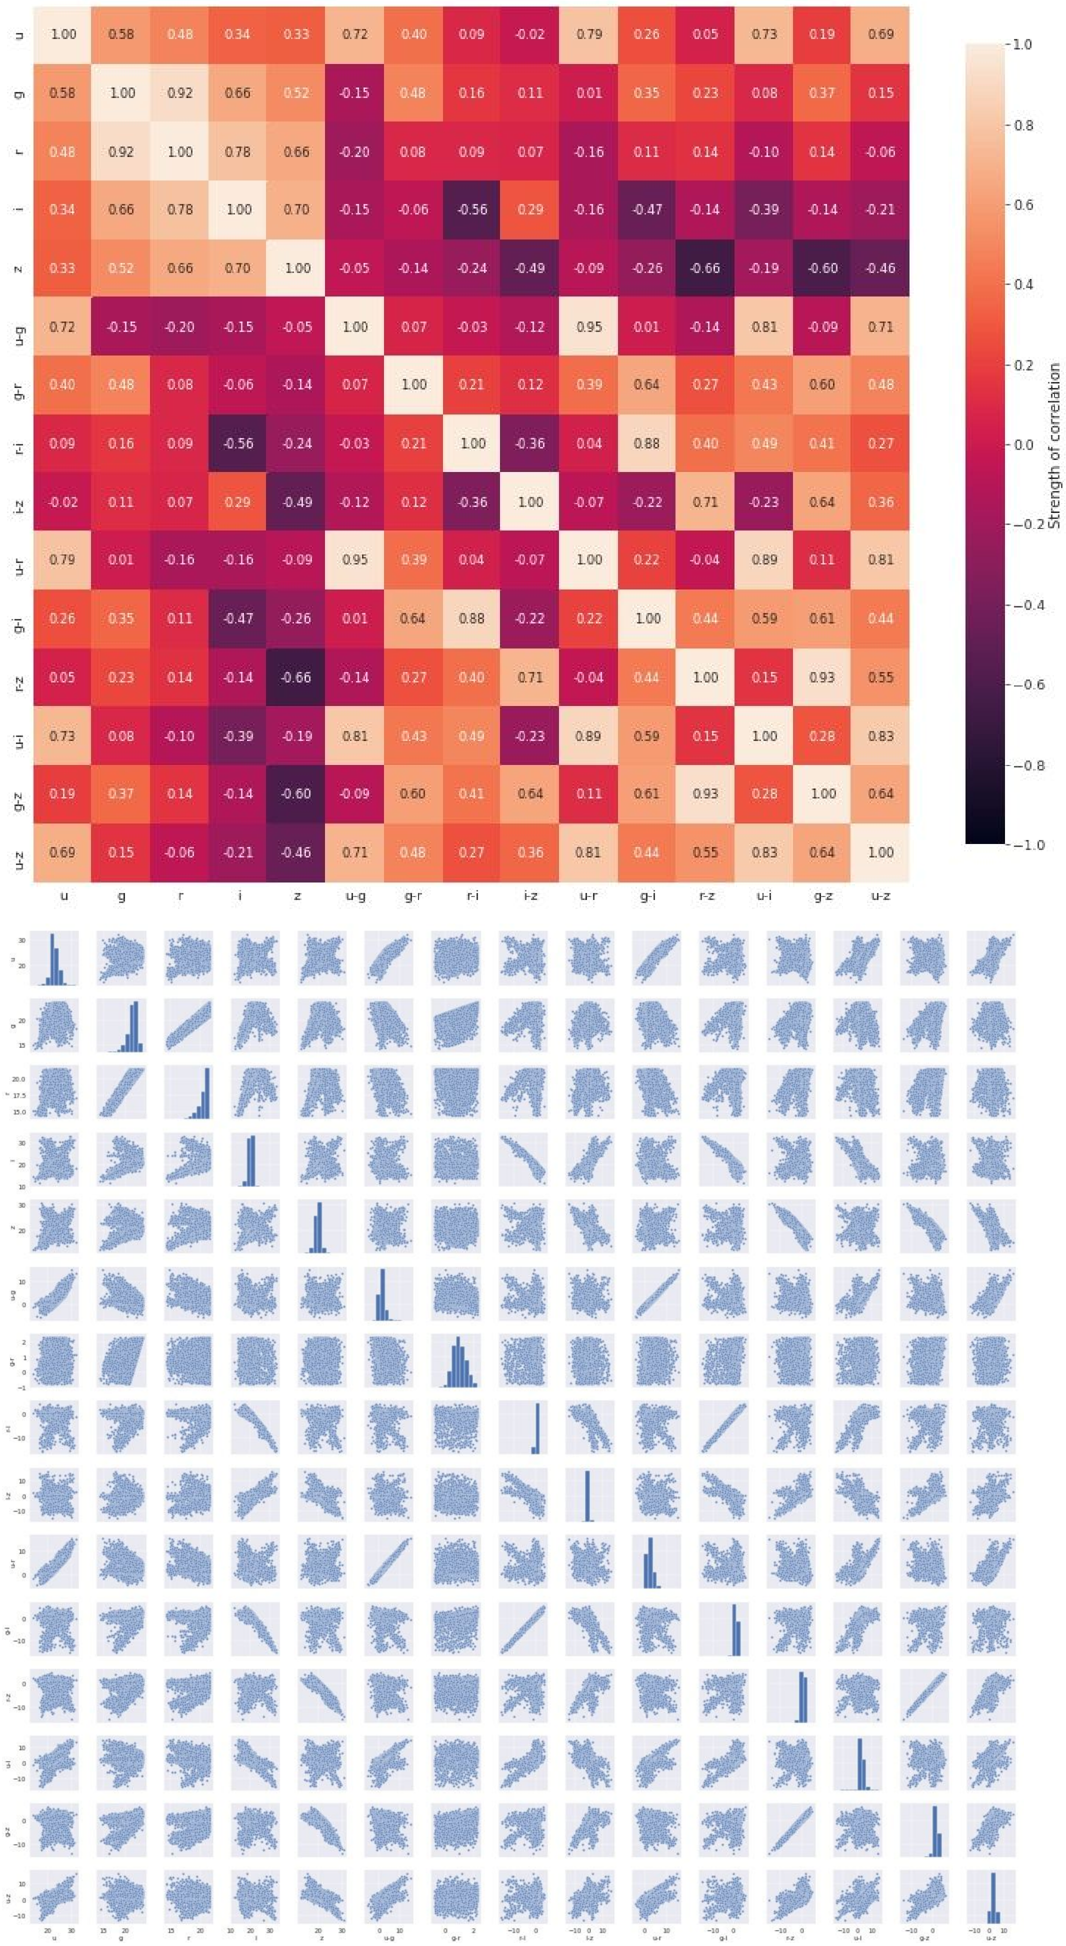


**Figure S4.** This figure is the same as Figure S3 except it is showing galaxies in our field galaxy sample.

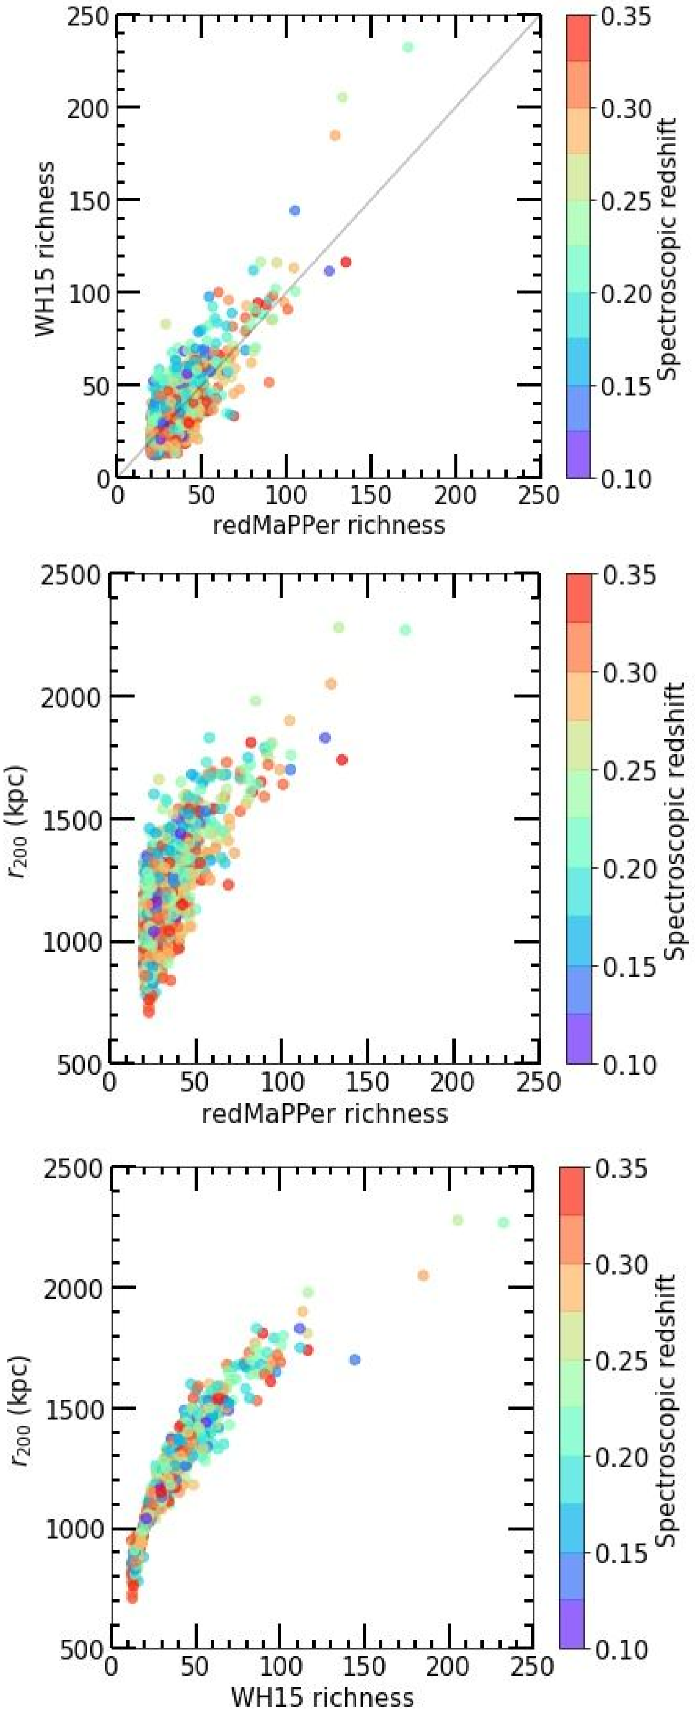


**Figure S5.** Top image: this figure displays a direct comparison between redMaPPer and WH15 richness for a subsample of cross-matched WH15 and redMaPPer clusters between a redshift range of $0.1 \leq z \leq 0.35$. Middle image: this figure displays a direct comparison between redMaPPer richness and $r_{200}$ values determined by WH15 for a subsample of cross-matched WH15 and redMaPPer clusters between a redshift range of $0.1 \leq z \leq 0.35$. Bottom image: this figure displays a direct comparison between WH15 richness and $r_{200}$ values determined by WH15 for a subsample of cross-matched WH15 and redMaPPer clusters between a redshift range of $0.1 \leq z \leq 0.35$.

| Random search iteration | Batch size | Learning rate | Optimiser algorithm | Architecture layout | AUCPR (per cent) [mean] | AUCPR (per cent) [standard deviation] |
|---|---|---|---|---|---|---|
| 1 | 512 | 0.0001 | 'RMSprop' | 5 | 39.87 | 1.52 |
| 2 | 2048 | 0.01 | 'Adadelta' | 1 | 34.03 | 2.46 |
| 3 | 2048 | 0.001 | 'Adam' | 5 | 38.93 | 1.27 |
| 4 | 1024 | 0.1 | 'Adadelta' | 5 | 38.94 | 2.14 |
| 5 | 512 | 0.001 | 'SGD' | 5 | 38.41 | 3.71 |
| 6 | 2048 | 0.0001 | 'Adagrad' | 3 | 33.68 | 1.22 |
| 7 | 256 | 0.001 | 'Adam' | 1 | 39.95 | 1.41 |
| 8 | 2048 | 0.0001 | 'Adadelta' | 1 | 34.02 | 0.35 |
| 9 | 256 | 0.1 | 'Adadelta' | 1 | 37.74 | 2.95 |
| 10 | 256 | 0.0001 | 'Adadelta' | 1 | 34.15 | 0.37 |
| 11 | 1024 | 0.001 | 'Adadelta' | 1 | 35.29 | 1.97 |
| 12 | 1024 | 0.0001 | 'Nadam' | 1 | 39.28 | 2.05 |
| 13 | 512 | 0.0001 | 'RMSprop' | 1 | 38.93 | 2.38 |
| 14 | 256 | 0.1 | 'Adadelta' | 5 | 39.18 | 1.30 |
| 15 | 1024 | 0.0001 | 'Nadam' | 5 | 39.23 | 2.36 |
| 16 | 256 | 0.01 | 'Adagrad' | 1 | 39.17 | 2.47 |
| 17 | 512 | 0.0001 | 'Nadam' | 3 | 38.65 | 1.63 |
| 18 | 512 | 0.1 | 'Nadam' | 1 | 34.08 | 0.34 |
| 19 | 1024 | 0.1 | 'Adam' | 3 | 35.82 | 3.34 |
| 20 | 2048 | 0.1 | 'SGD' | 5 | 38.48 | 1.51 |
| 21 | 1024 | 0.01 | 'Adagrad' | 3 | 39.00 | 3.01 |
| 22 | 256 | 0.1 | 'Nadam' | 5 | 34.08 | 0.34 |
| 23 | 1024 | 0.1 | 'Adamax' | 5 | 37.88 | 3.12 |
| 24 | 1024 | 0.0001 | 'Adadelta' | 3 | 33.74 | 0.98 |
| 25 | 2048 | 0.001 | 'RMSprop' | 1 | 39.50 | 2.07 |
| 26 | 1024 | 0.01 | 'Nadam' | 1 | 38.99 | 2.12 |
| 27 | 256 | 0.01 | 'Adadelta' | 3 | 38.89 | 1.69 |
| 28 | 512 | 0.001 | 'Nadam' | 3 | 39.51 | 1.43 |
| 29 | 512 | 0.01 | 'Adagrad' | 1 | 38.52 | 3.34 |
| 30 | 256 | 0.0001 | 'Adamax' | 3 | 38.05 | 1.25 |
| 31 | 512 | 0.001 | 'SGD' | 3 | 38.20 | 1.90 |
| 32 | 1024 | 0.1 | 'Adagrad' | 5 | 37.83 | 2.89 |
| 33 | 512 | 0.01 | 'Adamax' | 1 | 38.51 | 2.72 |
| 34 | 1024 | 0.01 | 'Adam' | 3 | 37.15 | 2.08 |
| 35 | 256 | 0.001 | 'Adagrad' | 1 | 36.44 | 2.80 |
| 36 | 1024 | 0.1 | 'Adadelta' | 3 | 38.08 | 2.24 |
| 37 | 2048 | 0.001 | 'Adadelta' | 1 | 33.83 | 2.25 |
| 38 | 256 | 0.1 | 'Adam' | 1 | 34.08 | 0.34 |
| 39 | 1024 | 0.0001 | 'Adagrad' | 5 | 34.09 | 1.48 |
| 40 | 512 | 0.01 | 'Adadelta' | 1 | 37.93 | 2.83 |
| 41 | 1024 | 0.0001 | 'Adamax' | 5 | 40.03 | 1.24 |
| 42 | 2048 | 0.0001 | 'Adam' | 5 | 39.26 | 2.00 |
| 43 | 256 | 0.01 | 'Nadam' | 5 | 39.15 | 2.27 |
| 44 | 2048 | 0.0001 | 'RMSprop' | 3 | 40.24 | 1.85 |
| 45 | 1024 | 0.1 | 'Nadam' | 5 | 34.08 | 0.34 |
| 46 | 512 | 0.0001 | 'Adam' | 5 | 37.64 | 2.09 |
| 47 | 2048 | 0.001 | 'Nadam' | 1 | 39.38 | 2.45 |
| 48 | 1024 | 0.1 | 'Nadam' | 3 | 34.08 | 0.34 |
| 49 | 512 | 0.1 | 'Adadelta' | 3 | 39.29 | 1.38 |
| 50 | 1024 | 0.0001 | 'RMSprop' | 1 | 39.36 | 2.19 |
| 51 | 2048 | 0.0001 | 'RMSprop' | 1 | 38.92 | 2.20 |
| 52 | 256 | 0.0001 | 'Adagrad' | 1 | 34.73 | 1.61 |
| 53 | 256 | 0.001 | 'SGD' | 1 | 37.09 | 2.16 |
| 54 | 1024 | 0.01 | 'RMSprop' | 1 | 37.56 | 3.23 |
| 55 | 512 | 0.001 | 'Adamax' | 5 | 38.17 | 2.19 |
| 56 | 1024 | 0.0001 | 'SGD' | 3 | 33.55 | 2.83 |
| 57 | 512 | 0.01 | 'SGD' | 5 | 38.79 | 2.05 |
| 58 | 1024 | 0.001 | 'SGD' | 1 | 34.61 | 3.00 |
| 59 | 1024 | 0.01 | 'Adadelta' | 5 | 37.68 | 1.74 |
| 60 | 256 | 0.01 | 'RMSprop' | 5 | 38.93 | 1.80 |

**Table S1.** This table displays the randomly selected hyper-parameter (i.e. batch size, learning rate, optimiser algorithm and architecture layout) combinations for tuning our background subtraction model on galaxies in our validation set using sixty iterations of random search. We also display the mean and standard deviation of the resultant AUCPR from performing ten iterations of Monte Carlo cross-validation on each random search iteration.

| Class probability threshold | F1 score (per cent) |
|---|---|
| 0 | 40.00 |
| 0.01 | 42.43 |
| 0.02 | 42.66 |
| 0.03 | 42.81 |
| 0.04 | 42.96 |
| 0.05 | 43.07 |
| 0.06 | 43.26 |
| 0.07 | 43.38 |
| 0.08 | 43.49 |
| 0.09 | 43.59 |
| 0.1 | 43.67 |
| 0.11 | 43.76 |
| 0.12 | 43.87 |
| 0.13 | 44.03 |
| 0.14 | 44.19 |
| 0.15 | 44.36 |
| 0.16 | 44.54 |
| 0.17 | 44.77 |
| 0.18 | 44.97 |
| 0.19 | 45.15 |
| 0.2 | 45.32 |
| 0.21 | 45.62 |
| 0.22 | 45.99 |
| 0.23 | 46.32 |
| 0.24 | 46.83 |
| 0.25 | 47.47 |
| 0.26 | 47.96 |
| 0.27 | 48.31 |
| 0.28 | 48.69 |
| 0.29 | 48.92 |
| 0.3 | 48.69 |
| 0.31 | 45.18 |
| 0.32 | 19.17 |
| 0.33 | 0.00 |
| 0.34 | 0.00 |
| 0.35 | 0.00 |
| 0.36 | 0.00 |
| 0.37 | 0.00 |
| 0.38 | 0.00 |
| 0.39 | 0.00 |
| 0.4 | 0.00 |
| 0.41 | 0.00 |
| 0.42 | 0.00 |
| 0.43 | 0.00 |
| 0.44 | 0.00 |
| 0.45 | 0.00 |
| 0.46 | 0.00 |
| 0.47 | 0.00 |
| 0.48 | 0.00 |
| 0.49 | 0.00 |
| 0.5 | 0.00 |
| 0.51 | 0.00 |
| 0.52 | 0.00 |
| 0.53 | 0.00 |
| 0.54 | 0.00 |
| 0.55 | 0.00 |
| 0.56 | 0.00 |
| 0.57 | 0.00 |
| 0.58 | 0.00 |
| 0.59 | 0.00 |
| 0.6 | 0.00 |
| 0.61 | 0.00 |
| 0.62 | 0.00 |
| 0.63 | 0.00 |
| 0.64 | 0.00 |
| 0.65 | 0.00 |
| 0.66 | 0.00 |
| 0.67 | 0.00 |
| 0.68 | 0.00 |
| 0.69 | 0.00 |
| 0.7 | 0.00 |
| 0.71 | 0.00 |
| 0.72 | 0.00 |
| 0.73 | 0.00 |
| 0.74 | 0.00 |
| 0.75 | 0.00 |
| 0.76 | 0.00 |
| 0.77 | 0.00 |
| 0.78 | 0.00 |
| 0.79 | 0.00 |
| 0.8 | 0.00 |
| 0.81 | 0.00 |
| 0.82 | 0.00 |
| 0.83 | 0.00 |
| 0.84 | 0.00 |
| 0.85 | 0.00 |
| 0.86 | 0.00 |
| 0.87 | 0.00 |
| 0.88 | 0.00 |
| 0.89 | 0.00 |
| 0.9 | 0.00 |
| 0.91 | 0.00 |
| 0.92 | 0.00 |
| 0.93 | 0.00 |
| 0.94 | 0.00 |
| 0.95 | 0.00 |
| 0.96 | 0.00 |
| 0.97 | 0.00 |
| 0.98 | 0.00 |
| 0.99 | 0.00 |
| 1 | 0.00 |

**Table S2.** This table displays the resultant F1 scores on galaxies in our validation set when using different class probability thresholds with the optimal hyper-parameter combination for our background subtraction model. It should be noted that an F1 score of 0 signifies that no cluster galaxies were identified at the given class probability threshold.

| Bin size | Chi-square fitting error | Number of bins with galaxies | M* | M* [standard deviation] | n* | n* [standard deviation] | α | α [standard deviation] |
|---|---|---|---|---|---|---|---|---|
| 0.01 | 102.140920976604 | 147 | -25.3072697006017 | 7.28783936301292 | 0.164112608931114 | 1.38199927866705 | -2 | 0.466629082092991 |
| 0.02 | 76.5453069917579 | 87 | -22.8960081024292 | 1.09379460105731 | 4.71921420366664 | 9.20338546553196 | -2 | 0.580632607165434 |
| 0.03 | 68.1745019597015 | 65 | -22.4908977078703 | 0.790075482406013 | 12.70439476778 | 18.952694149263 | -1.99999999999989 | 0.599104919143905 |
| 0.04 | 61.266861269483 | 50 | -22.415789304908 | 0.756339770593328 | 19.3568690083877 | 27.8274793059772 | -1.99999999999799 | 0.608973124211291 |
| 0.05 | 39.6185650543927 | 43 | -22.6222052707545 | 0.672513724488882 | 18.3176186296316 | 23.2838977629391 | -1.99999999999999 | 0.486524958545581 |
| 0.06 | 36.5625019331505 | 37 | -22.6258973735442 | 0.626947096373978 | 21.9653980090031 | 26.0819814894214 | -1.99999999999946 | 0.458571758087398 |
| 0.07 | 33.5900501761644 | 33 | -22.6099206948986 | 0.602242351450481 | 26.3737283301809 | 30.2193978863726 | -1.99999999998887 | 0.451033803392379 |
| 0.08 | 29.6385878283548 | 28 | -22.5816910642751 | 0.591756403834509 | 31.7971766662677 | 35.8707702408829 | -1.99999999999999 | 0.452169800589196 |
| 0.09 | 20.3637951180156 | 27 | -22.6746874027806 | 0.521101827728886 | 31.5718547496863 | 31.5686519817016 | -1.99999999999869 | 0.393056307595776 |
| 0.1 | 16.5530148685729 | 23 | -22.6582443109673 | 0.569061669900563 | 36.3423806202571 | 39.4465302657616 | -1.99999999999955 | 0.421022202247245 |
| 0.11 | 13.0767631976711 | 21 | -22.6755620489245 | 0.55251309291653 | 39.2543259599577 | 41.4152567582025 | -1.99999999999977 | 0.408316979552766 |
| 0.12 | 15.2459769970052 | 19 | -22.7247184161576 | 0.591396789212753 | 39.7619946638302 | 44.3787960605664 | -2 | 0.411200351509468 |
| 0.13 | 9.14827055635872 | 19 | -22.6183758110969 | 0.458502287321535 | 52.1384807705458 | 45.3748880546628 | -1.95453486711378 | 0.371591371552821 |
| 0.14 | 11.7492730266906 | 18 | -22.643331608495 | 0.462615820139636 | 52.7951370756613 | 47.0475807096035 | -1.98924101376699 | 0.367764744434002 |
| 0.15 | 10.9037429665667 | 16 | -22.4923685841581 | 0.448002369078026 | 74.7956455459639 | 61.8368875874148 | -1.88377867043106 | 0.397289759070223 |
| 0.16 | 16.7722783477289 | 15 | -22.5384337422092 | 0.475641293653476 | 70.5894407833445 | 64.5502898072399 | -1.97587961393189 | 0.404297179863603 |
| 0.17 | 4.15402355091424 | 15 | -22.7292157905515 | 0.466124335935932 | 56.9967978748963 | 51.1443097694934 | -2 | 0.351042953646424 |
| 0.18 | 12.7790690539623 | 14 | -22.6591309218703 | 0.490607883863879 | 65.8069565315428 | 62.2084888857685 | -1.99999999999884 | 0.381498515390209 |
| 0.19 | 10.1521887967407 | 13 | -22.7126392343591 | 0.531049352235773 | 64.521848195881 | 65.4523309529134 | -2 | 0.389521040297862 |
| 0.2 | 7.99147466406507 | 12 | -22.7208482829558 | 0.537766203637089 | 67.4775596294566 | 69.1927939236387 | -2 | 0.390696836606222 |
| 0.21 | 4.29404454893266 | 12 | -22.7778047368944 | 0.507161177536059 | 65.6184421027745 | 63.563335472533 | -2 | 0.363575936524285 |
| 0.22 | 5.67230887264036 | 11 | -22.7623890236569 | 0.525989016830309 | 70.1952555544012 | 70.3336011457905 | -2 | 0.374685241450145 |
| 0.23 | 3.92256129130857 | 11 | -22.705216487009 | 0.489026439161547 | 80.1076053301875 | 75.3087082850019 | -2 | 0.369199150776928 |
| 0.24 | 8.17416297511997 | 10 | -22.5708249356802 | 0.46728589789064 | 104.425526335234 | 92.3190354948186 | -1.94542652350871 | 0.390175180596096 |
| 0.25 | 4.29832445617372 | 10 | -22.7749629261976 | 0.504034834908083 | 78.5599805972613 | 75.5810214476751 | -1.99999999999975 | 0.360888114340128 |
| 0.26 | 1.5900013241842 | 10 | -22.7543979409332 | 0.456121860305321 | 84.6673328318602 | 74.3374090694452 | -2 | 0.340403198275327 |
| 0.27 | 4.97043601393654 | 9 | -22.7326239407067 | 0.537509637953644 | 90.2958645221638 | 92.7197761899969 | -2 | 0.390545267175811 |
| 0.28 | 4.10694483459387 | 9 | -22.7361583932848 | 0.475351264466895 | 94.4841506940494 | 85.5761639766845 | -1.97909263203428 | 0.356655435560158 |
| 0.29 | 2.43440108474398 | 9 | -22.7735764454752 | 0.483748588363934 | 91.7522170908038 | 85.1097978159416 | -2 | 0.353263598483103 |
| 0.3 | 5.15205257540701 | 8 | -22.7918350993829 | 0.571519770757192 | 92.0936083899066 | 99.5684604796216 | -2 | 0.393299649494388 |
| 0.31 | 5.90218198017966 | 8 | -22.7496055699693 | 0.512441830655374 | 101.027295842528 | 99.0607465472664 | -1.99999999999849 | 0.374980540977817 |
| 0.32 | 10.1014409330581 | 8 | -22.7068155761029 | 0.46673483659344 | 110.104060272333 | 99.3073073368942 | -2 | 0.361982802750744 |
| 0.33 | 5.96846341699309 | 8 | -22.7391063048754 | 0.46925404584864 | 109.201691285243 | 98.8710176390871 | -2 | 0.356791209942564 |
| 0.34 | 1.12105000461229 | 8 | -22.7478245333539 | 0.440292188347238 | 112.250370963957 | 95.4874446889144 | -2 | 0.336758675291583 |
| 0.35 | 3.12523238008784 | 7 | -22.7822285687626 | 0.546318661436639 | 109.623965612747 | 113.882723095951 | -1.9999999999999 | 0.387253819700969 |
| 0.36 | 3.03061687353762 | 7 | -22.7241788039726 | 0.52765200413997 | 122.841382114879 | 123.931590655044 | -2 | 0.390054298402819 |
| 0.37 | 1.48984677624025 | 7 | -22.7309176072148 | 0.46076140879309 | 125.422731293451 | 111.639466908686 | -2 | 0.354493289723339 |
| 0.38 | 2.36115567803497 | 7 | -22.758776999429 | 0.469319697928797 | 123.406631037008 | 111.329064686043 | -2 | 0.350817563549449 |
| 0.39 | 0.603516773400222 | 7 | -22.6964112181343 | 0.413245262968147 | 140.371839664555 | 112.444496886239 | -1.98962179171752 | 0.334505631972704 |
| 0.4 | 0.637438766276678 | 6 | -22.7621355562676 | 0.547164384340818 | 130.14248212713 | 135.853063636089 | -2 | 0.394672140845081 |
| 0.41 | 1.03851432178477 | 6 | -22.7388960765666 | 0.539100941022473 | 137.925294842631 | 142.459296913682 | -1.9999999999998 | 0.398317582214352 |
| 0.42 | 0.617019282021179 | 6 | -22.7836403833345 | 0.52063968702413 | 132.412600884289 | 131.908715973817 | -2 | 0.377789372068514 |
| 0.43 | 1.00222006125957 | 6 | -22.7669424142399 | 0.497083941926808 | 138.844175703839 | 132.560878756468 | -2 | 0.368534172557065 |
| 0.44 | 1.3854524348229 | 6 | -22.735461750642 | 0.442508674389626 | 149.866239382466 | 127.730806309675 | -1.98775443119698 | 0.344888791011023 |
| 0.45 | 2.09325476913197 | 6 | -22.7542533890697 | 0.455514311827121 | 147.815629869087 | 129.964796940122 | -2 | 0.347242980067736 |
| 0.46 | 2.06708478166107 | 6 | -22.7198920761451 | 0.449235034517127 | 159.112883886869 | 138.59783627731 | -2 | 0.353667237181105 |
| 0.47 | 1.91277317747975 | 6 | -22.7134175644432 | 0.4158846753342 | 164.305815020088 | 133.021223122312 | -1.99999999999996 | 0.33502131248639 |
| 0.48 | 3.09959702941975 | 5 | -22.7133128234714 | 0.526534407663765 | 168.666330230149 | 170.028242094597 | -1.991839331825 | 0.400161540375978 |
| 0.49 | 2.99396275206369 | 5 | -22.7586216420838 | 0.530865270015062 | 160.296570599804 | 163.000668703465 | -1.99999999999998 | 0.391406599797717 |
| 0.5 | 3.01068130899773 | 5 | -22.7996514653902 | 0.532221118709986 | 154.04407380113 | 156.784199434023 | -1.99999999999812 | 0.383433470402977 |
| 0.51 | 1.10735348985882 | 5 | -22.8207986936304 | 0.529542207845286 | 153.028828033463 | 154.869239126894 | -1.99999999999999 | 0.37851641868231 |
| 0.52 | 0.566621255611028 | 5 | -22.8082232056862 | 0.504804314046596 | 159.821770266413 | 154.624246072466 | -1.99360356962263 | 0.370844073513688 |
| 0.53 | 0.804364552288225 | 5 | -22.5216510211879 | 0.418951220094654 | 274.838166240616 | 202.702584893226 | -1.77308302024065 | 0.391484698263154 |
| 0.54 | 2.39612065033725 | 5 | -22.5437634518665 | 0.441778546861592 | 265.78170850412 | 210.927359077781 | -1.8183753728052 | 0.401173098435923 |
| 0.55 | 1.46317886420762 | 5 | -22.4701482130265 | 0.382373057404958 | 310.083447783411 | 206.11140981392 | -1.74205611806367 | 0.377492189289949 |
| 0.56 | 1.51574912980039 | 5 | -22.5086962590682 | 0.39050000766944 | 297.455379636805 | 203.562572401559 | -1.75836724883236 | 0.375135903611389 |
| 0.57 | 1.45663254988623 | 5 | -22.5602264810274 | 0.402236411508689 | 278.002178944076 | 199.230027703658 | -1.79306653623351 | 0.372083907644912 |
| 0.58 | 0.719369820743466 | 5 | -22.6910262019285 | 0.426822999134624 | 223.608144930381 | 178.401952889802 | -1.90202692521294 | 0.3585602913609 |
| 0.59 | 0.589469793678187 | 5 | -22.603110886294 | 0.376524243377872 | 267.158181157209 | 183.285827177277 | -1.83213557762778 | 0.345949650208558 |

**Table S3.** This table displays the computed Chi-square fitting errors when fitting the Schechter function to a composite luminosity distribution that consisted of a subsample of identified cluster galaxies from our CMWR-$r_{200}$ training set that visually appeared to have high completeness. We also display the best fit parameter values for $M*$, $n*$ and $a$ as well as their respective standard deviations when using different $r$ filter absolute magnitude bin sizes. In addition, we display the number of bins that contain at least one identified cluster galaxy. It should be noted that we do not display the results of bin sizes that have fewer than five bins with identified cluster galaxies nor do we display the results of bin sizes that do not have successful fits.
